# Supplementary material for: Enhancing Node Representations for Real-World Complex Networks with Topological Augmentation
Source: arXiv:2402.13033 source file (2024-08-12)
Supplement: Supplementary file 1 [file data-access.tex]

\section{Code and Data Accessibility}

The source code and full datasets of SHGB is publicly available at \url{https://anonymous-url/}. %\url{https://zehui127.github.io/hybrid-graph-benchmark/}. 
While the raw dataset in JSON format is hosted at \url{https://anonymous-url/}, %\url{https://zenodo.org/record/7982540}, 
we recommend the users to access the datasets through our Python library \texttt{anonymous-library}, %\texttt{hybrid-graph}, 
which is installable via \texttt{pip}. This would allow the users to read the graphs in the format of PyTorch Geometric \texttt{Data} objects.
